# Supplementary material for: How long, O Bayesian network, will I sample thee? A program analysis perspective on expected sampling times
Source: arXiv:1802.10433 source file (2018-02-28)
Supplement: Supplementary file 1 [file appendix.tex]

% !TEX root = ./main.tex

\subsection{Calculation for Expected Sampling Time of Example Network}
%Macros for variables associated to nodes:
\newcommand{\vNodeR}{x_{\nodeR}}
\newcommand{\vNodeS}{x_{\nodeS}}
\newcommand{\vNodeG}{x_{\nodeG}}
\newcommand{\bnlExampleLoopBody}{C}
Let $\BN$ denote the Bayesian Network shown in Figure~\ref{fig:intro:bn}. We denote the nodes by $\nodeR$, $\nodeS$, and $\nodeG$, respectively. 
Since we want to condition $\nodeG$ to value $0$, let $\BNCOND (\nodeG)=0$, $\BNCOND (\nodeR)=\bot$, and $\BNCOND (\nodeS)=\bot$.
According to the translation from Bayesian Networks to $\bnl$ programs presented in Section~\ref{sec:bnl}, we obtain the following
program $\TBN{\BN}{\BNCOND}$:
\begin{align*}
       &\mathtt{repeat} \{ \\
       &\qquad //~ \text{translation of node $\nodeR$, denoted $\TNODE{\BN}{\nodeR}{\BNCOND}$} \\
       &\qquad \PASSIGN{\vNodeR}{a \cdot \langle 0 \rangle + (1-a) \cdot \langle 1 \rangle};\\
       &\qquad \phantom{aa} \\
       &\qquad //~ \text{translation of node $\nodeS$, denoted $\TNODE{\BN}{\nodeS}{\BNCOND}$} \\
       &\qquad \IFBRACK{\vNodeR = 0} \\
       &\qquad \qquad \PASSIGN{\vNodeS}{a \cdot \langle 0 \rangle + (1-a) \cdot \langle 1 \rangle} \\ 
       &\qquad \} ~\ELSE~ \{ \\
       &\qquad \qquad \PASSIGN{\vNodeS}{0.2 \cdot \langle 0 \rangle + 0.8 \cdot \langle 1 \rangle} \}; \\
       &\qquad \phantom{aa} \\
       &\qquad //~ \text{translation of node $\nodeG$, denoted $\TNODE{\BN}{\nodeG}{\BNCOND}$} \\
       &\qquad \IFBRACK{\vNodeS =0 \wedge \vNodeR =0} \\ 
       &\qquad \qquad  \PASSIGN{\vNodeG}{0.01 \cdot \langle 0 \rangle + (0.99 \cdot \langle 1 \rangle} \\  
       &\qquad \}~ \ELSE \IFBRACK{\vNodeS =0 \wedge \vNodeR =1} \\
       &\qquad \qquad  \PASSIGN{\vNodeG}{0.25 \cdot \langle 0 \rangle + (0.75 \cdot \langle 1 \rangle}\\
       &\qquad  \}~ \ELSE \IFBRACK{\vNodeS =1 \wedge \vNodeR =0} \\
       &\qquad \qquad  \PASSIGN{\vNodeG}{0.9 \cdot \langle 0 \rangle + (0.1 \cdot \langle 1 \rangle} \\
       &\qquad \}~ \ELSE~ \{ \\
       &\qquad \qquad  \PASSIGN{\vNodeG}{0.2 \cdot \langle 0 \rangle + (0.8 \cdot \langle 1 \rangle} \}\\
       &\}\mathtt{until}\left(\vNodeG = 0 \right) // \text{condition node $\nodeG$ to value $0$}
\end{align*}
Thus we have
\begin{align*}
       &\ert{\TBN{\BN}{\BNCOND}}{0} \\
       &{}={}~ \ert{\REPEATUNTIL{\COMPOSE{\COMPOSE{\TNODE{\BN}{\nodeR}{\BNCOND}}{\TNODE{\BN}{\nodeS}{\BNCOND}}}{\TNODE{\BN}{\nodeG}{\BNCOND}}}{\vNodeG = 0}}{0}~. 
\end{align*} 
Let 
$\bnlExampleLoopBody$ denote the body of the above loop. Theorem~\ref{thm:bnl:repeat} then yields
\begin{align*}
       \ert{\REPEATUNTIL{\bnlExampleLoopBody}{\vNodeG = 0}}{0} ~{}={}~ \frac{1+ \ert{\bnlExampleLoopBody}{0}}{\wp{\bnlExampleLoopBody}{\iverson{\vNodeG = 0}}}~.
\end{align*}
We first compute $\ert{C}{0} = \ert{\COMPOSE{\COMPOSE{\TNODE{\BN}{\nodeR}{\BNCOND}}{\TNODE{\BN}{\nodeS}{\BNCOND}}}{\TNODE{\BN}{\nodeG}{\BNCOND}}}{0}$. We have
\begin{align*}
      \ert{\TNODE{\BN}{\nodeG}{\BNCOND}}{0} ~{}={}~ 2 + \iverson{\vNodeS \neq 0 \vee \vNodeR \neq 0} \cdot \left(1 + \iverson{\vNodeS \neq 0 \vee \vNodeR \neq0} \right)~,
\end{align*}
thus
\begin{align*}
       \ert{\TNODE{\BN}{\nodeS}{\BNCOND}}{\ert{\TNODE{\BN}{\nodeG}{\BNCOND}}{0}} ~{}={}~ \frac{18}{5} + \iverson{\vNodeR = 0} \cdot \left( \frac{2}{5} - 2a \right)~,
\end{align*}
and finally
\begin{align*}
       &\ert{C}{0} \\
       &{}={}~ \ert{\TNODE{\BN}{\nodeR}{\BNCOND}}{\ert{\TNODE{\BN}{\nodeS}{\BNCOND}}{\ert{\TNODE{\BN}{\nodeG}{\BNCOND}}{0}}} \\
       &{}={}~ -2a^2 + \frac{2}{5} a + \frac{18}{5}~.
\end{align*}
Next, we determine $\wp{\bnlExampleLoopBody}{\iverson{\vNodeG = 0}}$ and therefore calculate
\begin{align*}
      \wp{\TNODE{\BN}{\nodeG}{\BNCOND}}{\iverson{\vNodeG = 0}} 
      &{}={}~ 0.01 \cdot \iverson{\vNodeS =0 \wedge \vNodeR =0}  + 0.25 \cdot \iverson{\vNodeS = 0 \wedge \vNodeR = 1} \\
      &\qquad + 0.9 \cdot \iverson{\vNodeS = 1 \wedge \vNodeR = 0}
              + 0.2 \cdot \iverson{\vNodeS = 1 \wedge \vNodeR = 1}~,
\end{align*}
and
\begin{align*}
       &\wp{\TNODE{\BN}{\nodeS}{\BNCOND}}{\wp{\TNODE{\BN}{\nodeG}{\BNCOND}}{0}} \\
       &{}={}~ \frac{21}{100} + \iverson{\vNodeR = 0} \cdot \left(- \frac{89}{100} a + \frac{69}{100} \right)~,
\end{align*}
thus we finally obtain
\begin{align*}
       &\wp{C}{\iverson{\vNodeG = 0}} \\
       &{}={}~ \wp{\TNODE{\BN}{\nodeR}{\BNCOND}}{\wp{\TNODE{\BN}{\nodeS}{\BNCOND}}{\wp{\TNODE{\BN}{\nodeG}{\BNCOND}}{\iverson{\vNodeG = 0}}}} \\
       &{}={}~ -\frac{89}{100} a^2 + \frac{69}{100} a + \frac{21}{100}~.
\end{align*}
Overall, by applying some simple algebra, we get
\begin{align*}
       \ert{\REPEATUNTIL{\bnlExampleLoopBody}{\vNodeG = 0}}{0} ~{}={}~ \frac{200a^2 - 40a - 460}{89a^2 -69a -21}~.
\end{align*}

\subsection{Proof of Lemma~\ref{lem:oldrule_wp_finite_approximations}}
\label{proof-lem:oldrule_wp_finite_approximations}
In order to derive a characterization of the $\wpsymbol$--semantics of an universally i.i.d.\ loop's finite approximations, we define
\begin{align*}
	\wpFold{C}{f}{g}{0} = \wp{C}{f} \qqand \wpFold{C}{f}{g}{n+1} = \wp{C}{g \cdot \wpFold{C}{f}{g}{n}}~.
\end{align*}
Furthermore, we require the following lemma.
\begin{lemma}
       \label{lem:oldrule_technical}
       Let $C \in \pgcl$ and $\kGuard$ be a guard such that the loop $\WHILEDO{\kGuard}{C}$ is universally
       independent and identically distributed. Then for all $i \in \Nats$ and all $f \in \E$, we have
       \begin{equation*}
              \wpFold{C}{f}{\iverson{\kGuard}}{i} \eeq \wp{C}{f} \cdot \wp{C}{\iverson{\kGuard}}^i~.
       \end{equation*} 
\end{lemma}
\begin{proof}
       By induction on $i$. We consider the cases $i=0$ and $i=1$ as the induction base. 
       For $i=0$, we have
       \begin{equation*}
		\wpFold{C}{f}{\iverson{\kGuard}}{0} \eeq \wp{C}{f} \eeq \wp{C}{f} \cdot \underbrace{\wp{C}{\iverson{\kGuard}}^0}_{{}=1}~.
       \end{equation*}
       For $i=1$, we have
       \begin{align*}
		\wpFold{C}{f}{\iverson{\kGuard}}{1} & \eeq \wp{C}{\iverson{\kGuard} \cdot  \wp{C}{f}} 
        \\
		& \eeq \wp{C}{f} \cdot \wp{C}{\iverson{\kGuard}}^1  \tag {by universal i.i.d.--ness, see Definition~\ref{def:iid}}~.
       \end{align*}

       As the induction hypothesis we now assume the lemma holds for some arbitrary but fixed $i  > 1$.
       
       For the induction step, we have
       \begin{align*}
               \wpFold{C}{f}{\iverson{\kGuard}}{i+1} 
               &\eeq  \wp{C}{\iverson{\kGuard} \cdot  \wp{C}{\underbrace{\iverson{\kGuard} \cdot \wpFold{C}{f}{\iverson{\kGuard}}{i-1}}_{{}\eqqcolon f'}}} \\
               &\eeq  \wp{C}{\underbrace{\iverson{\kGuard} \cdot \wpFold{C}{f}{\iverson{\kGuard}}{i-1}}_{f'}} \cdot \wp{C}{\iverson{\kGuard}} \tag{by universal i.i.d.--ness applied to $f'$, see Definition~\ref{def:iid}} \\
               &\eeq \wpFold{C}{f}{\iverson{\kGuard}}{i} \cdot \wp{C}{\iverson{\kGuard}} \\
               &\eeq \wp{C}{f} \cdot \wp{C}{\iverson{\kGuard}}^{i} \cdot \wp{C}{\iverson{\kGuard}} \tag{by I.H.\ } \\
               &\eeq \wp{C}{f} \cdot \wp{C}{\iverson{\kGuard}}^{i+1}~.\tag*{\qed}
       \end{align*}
\end{proof}
The probability of the guard evaluating to $\true$ after one iteration is given by $\wp{C}{\kGuardB}$. The lemma above states that the events 
``loop guard $\kGuard$ evaluates to $\true$ after iteration $i$" are independent. Thus the probability of their union, i.e. ``loop guard $\kGuard$ evaluates to true after iterations $1$ to $i$" is 
given by the product of their probabilities $\wp{C}{\kGuardB}^i$. The fact that $\wp{C}{f}$ is also independent of these events for all $f\in \E$ results in the lemma, which is used in the following proof.

\begin{proof}
       By induction on $n$. We consider the cases $n=1$ and $n=2$ as the induction base.
       For $n=1$, we have
       \begin{align}
              \wp{\WHILEDOapprox{\kGuard}{C}{1}}{f} &~{}={}~ \wp{\ITE{\kGuard}{\COMPOSE{C}{\WHILEDOapprox{\kGuard}{C}{0}}}{\SKIP}}{f}
              \tag{by Definition~\ref{def:finite_approximations}} \\
              &~{}={}~ \wp{\ITE{\kGuard}{\COMPOSE{C}{\DIVERGE}}{\SKIP}}{f} \tag{by Definition~\ref{def:finite_approximations}} \\
              &~{}={}~ \iverson{\kGuard} \cdot \wp{C}{0} + \iverson{\neg \kGuard} \cdot f \tag{by \autoref{table:wp}} \\
              &~{}={}~ \iverson{\kGuard} \cdot 0 + \iverson{\neg \kGuard} \cdot f \tag{by strictness, see Theorem~\ref{thm:basic-prop} (\ref{thm:basic-prop-strictness})} \\
              &~{}={}~ \iverson{\neg \kGuard} \cdot f \label{eqn:while_one} \\
              &~{}={}~ \iverson{\kGuard} \cdot 0 + \iverson{\neg \kGuard} \cdot f \notag \\
              &~{}={}~ \iverson{\kGuard} \cdot \wp{C}{\iverson{\neg \kGuard} \cdot f}
               \cdot \underbrace{\left. \sum\limits_{i=0}^{-1} \middle(\wp{C}{\iverson{\kGuard}}^i \right)}_{{}=0} + \iverson{\neg \kGuard} \cdot f~. 
               \notag
       \end{align}
       For $n=2$, we have
       \begin{align*}
        \wp{\WHILEDOapprox{\kGuard}{C}{2}}{f} &~{}={}~
              \wp{\ITE{\kGuard}{\COMPOSE{C}{\WHILEDOapprox{\kGuard}{C}{1}}}{\SKIP}}{f}
              \tag{by Definition~\ref{def:finite_approximations}} \\
              &~{}={}~ \iverson{\kGuard} \cdot \wp{C}{\wp{\WHILEDOapprox{\kGuard}{C}{1}}{f}} + \iverson{\neg \kGuard} + f  \tag{by \autoref{table:wp}} \\
              &~{}={}~ \iverson{\kGuard} \cdot \wp{C}{\iverson{\neg \kGuard} \cdot f} + \iverson{\neg \kGuard} \cdot f
              \tag{by \autoref{eqn:while_one}} \\
              &~{}={}~ \iverson{\kGuard} \cdot  \wp{C}{\iverson{\neg \kGuard} \cdot f}
               \cdot \underbrace{\left. \sum\limits_{i=0}^{0} \middle( \wp{C}{\iverson{\kGuard}}^i \right)}_{{}=1} + \iverson{\neg \kGuard} \cdot f~.
       \end{align*}
       Before we perform the inductive step, observe that the following equality holds for all $n \in \Nats$ and $f \in E$:
       \begin{align}
       &\wp{C}{\iverson{\kGuard} \cdot \wp{C}{\iverson{\neg \kGuard} \cdot f}
       \cdot \left. \sum\limits_{i=0}^{n-2} \middle(\wp{C}{\iverson{\kGuard}}^i\right)} \notag \\
       &{}={}~ \left.\sum\limits_{i=0}^{n-2} \middle( \wp{C}{\iverson{\kGuard} \cdot \wp{C}{\iverson{\neg \kGuard} \cdot f}
       \cdot \wp{C}{\iverson{\kGuard}}^i} \right) \tag{by linearity, see Theorem~\ref{thm:basic-prop} (\ref{thm:basic-prop-linearity})} \\
       &{}={}~ \left. \sum\limits_{i=0}^{n-2} \middle( \wp{C}{\iverson{\kGuard} 
       \cdot \wpFold{C}{\iverson{\neg \kGuard} \cdot f}{\iverson{\kGuard}}{i}} \tag{by Lemma~\ref{lem:oldrule_technical}}\right) \notag \\
       &{}={}~ \left. \sum\limits_{i=0}^{n-2} \middle(\wp{C}{\iverson{\kGuard}} \cdot
       \wpFold{C}{\iverson{\neg \kGuard} \cdot f}{\iverson{\kGuard}}{i} \right) \tag{by universal i.i.d.--ness, see Definition~\ref{def:iid}} \\
       &{}={}~ \left. \sum\limits_{i=0}^{n-2} \middle(\wp{C}{\iverson{\kGuard}} \cdot \wp{C}{\iverson{\neg \kGuard} \cdot f}
       \cdot \wp{C}{\iverson{\kGuard}}^i \right) \tag{by Lemma~\ref{lem:oldrule_technical}} \\
       &{}={}~ \wp{C}{\iverson{\kGuard}} \cdot \wp{C}{\iverson{\neg \kGuard} \cdot f}
       \cdot \left. \sum\limits_{i=0}^{n-2}  \middle(\wp{C}{\iverson{\kGuard}}^i \right) \label{eqn: oldrule-semantics-proof}
       \end{align}
       We now assume the lemma holds for some arbitrary but fixed $n \in \Nats \setminus \{ 0 \}$. 
       We calculate
       \begin{align*}
       &\wp{\WHILEDOapprox{\kGuard}{C}{n+1}}{f} \\
       &{}={}~ \wp{\ITE{\kGuard}{\COMPOSE{C}{\WHILEDOapprox{\kGuard}{C}{n}}}{\SKIP}}{f}
                    \tag{By Definition \ref{def:finite_approximations}} \\
       &{}={}~ \iverson{\kGuard} \cdot \wp{C}{\wp{\WHILEDOapprox{\kGuard}{C}{n}}{f}} 
                    + \iverson{\neg \kGuard} \cdot f
                    \tag{by Table~\ref{table:wp}} \\
       &{}={}~ \iverson{\kGuard} \cdot \wp{C}{ \iverson{\kGuard} \cdot \wp{C}{\iverson{\neg \kGuard} \cdot f}
                    \cdot \left. \sum\limits_{i=0}^{n-2}\middle( \wp{C}{\iverson{\kGuard}}^i \right)+ \iverson{\neg \kGuard} \cdot f}
                    + \iverson{\neg \kGuard} \cdot f
       \tag{by I.H.} \\
       &{}={}~ \iverson{\kGuard} \cdot \left( ~\underbracket{\wp{C}{\iverson{\kGuard} \cdot \wp{C}{\iverson{\neg \kGuard} \cdot f}
                    \cdot \left. \sum\limits_{i=0}^{n-2}\middle( \wp{C}{\iverson{\kGuard}}^i \right)}}_{\text{see Equation \ref{eqn: oldrule-semantics-proof}}}
                    {}+ \wp{C}{\iverson{\neg \kGuard} \cdot f} \right) + \iverson{\neg \kGuard} \cdot f
                    \tag{by linearity, see Theorem~\ref{thm:basic-prop} (\ref{thm:basic-prop-linearity})} \\
       &{}={}~  \iverson{\kGuard} \cdot \left( ~\underbracket{\wp{C}{\iverson{\kGuard}} \cdot \wp{C}{\iverson{\neg \kGuard} \cdot f}
                     \cdot \left. \sum\limits_{i=0}^{n-2} \middle(  \wp{C}{\iverson{\kGuard}}^i \right)}_{\text{see Equation \ref{eqn: oldrule-semantics-proof}}}
                  {} + \wp{C}{\iverson{\neg \kGuard} \cdot f} \right) + \iverson{\neg \kGuard} \cdot f
                     \tag{By Equation \ref{eqn: oldrule-semantics-proof}} \\
       &{}={}~  \iverson{\kGuard} \cdot \left(\wp{C}{\iverson{\neg \kGuard} \cdot f}
                     \cdot \left. \sum\limits_{i=1}^{n-1} \middle(  \wp{C}{\iverson{\kGuard}}^i \right)
                  + \wp{C}{\iverson{\neg \kGuard} \cdot f} \right) + \iverson{\neg \kGuard} \cdot f \\
       &{}={}~  \iverson{\kGuard} \cdot \wp{C}{\iverson{\neg \kGuard} \cdot f}
                     \cdot \left. \sum\limits_{i=0}^{n-1} \middle( \wp{C}{\iverson{\kGuard}}^i  \right) 
                     + \iverson{\neg \kGuard} \cdot f ~.\tag*{\qed}
       \end{align*}
\end{proof}

\subsection{Proof of Lemma~\ref{lem:oldrule-technical-three}}
\label{proof-lem:oldrule-technical-three}
\begin{proof}
       By induction on $n$. As the induction base we consider the cases $n=0$ and $n=1$.
       For $n=0$, we have
       \begin{equation*}
              \wp{C}{\kGuardB} \cdot \underbrace{\wp{C}{\kGuardB}^0}_{{}=1} \eeq  
              \wp{C}{\kGuardB \cdot \underbrace{\wp{C}{\kGuardB}^0}_{{}=1}}~.
       \end{equation*}
       For $n=1$, we have
       \begin{align*}
              \wp{C}{\kGuardB} \cdot \wp{C}{\kGuardB}^1 \eeq 
              \wp{C}{\kGuardB \cdot \wp{C}{\kGuardB}} \tag{by universal i.i.d.--ness, see Definition \ref{def:iid}}~.
       \end{align*}

       As the induction hypothesis we assume that the lemma holds for some arbitrary but fixed
       $n \in \Nats$ with $n>0$. 
       
       For the induction step, we calculate
       \begin{align*}
                        \wp{C}{\kGuardB} \cdot \wp{C}{\kGuardB}^{n+1} 
	& \eeq 
                        \wp{C}{\kGuardB} \cdot \wp{C}{\kGuardB}^{n} \cdot \wp{C}{\kGuardB} \\
        &\eeq   \wp{C}{\underbrace{\kGuardB \cdot \wp{C}{\kGuardB}^n}_{{}\eqqcolon f'}} \cdot \wp{C}{\kGuardB} 
                        \tag{by I.H.} \\
        &\eeq   \wp{C}{\kGuardB \cdot \wp{C}{\underbrace{\kGuardB \cdot \wp{C}{\kGuardB}^n}_{f'}}}          
                        \tag{by universal i.i.d.--ness applied on $f'$, see Definition \ref{def:iid}} \\
        &\eeq  \wp{C}{\kGuardB \cdot \wp{C}{\kGuardB} \cdot \wp{C}{\kGuardB}^{n}}      
                       \tag{by I.H.} \\        
        &\eeq  \wp{C}{\kGuardB \cdot \wp{C}{\kGuardB}^{n+1}}~.\tag*{\qed}                  
       \end{align*}
\end{proof}
\noindent
\subsection{Proof of Theorem~\ref{thm:oldrule-proof-rule}}
\label{proof-thm_oldrule-proof-rule}
In order to prove Theorem~\ref{thm:oldrule-proof-rule}, we provide a lower and upper $\omega$--invariant for universally i.i.d.\ loops and analyze
its asymptotic behavior. Proving the $\omega$--invariant correct requires the following technical corollary.
\begin{corollary}
       \label{cor:oldrule-technical-two}
       Let $C \in \pgcl$ and $\kGuard$ be a guard such that the loop $\WHILEDO{\kGuard}{C}$ is
       universally independent and identically distributed. Furthermore assume 
       \begin{equation}
              \label{eqn:oldrule-technical-two}
              \wp{C}{\ert{C}{0}} = \ert{C}{0}~.
       \end{equation}
       Then the following equation holds for all $n \in \Nats$:
       \begin{equation*}
              \ert{C}{0} \cdot \wp{C}{\kGuardB}^n = \wpFold{C}{\ert{C}{0}}{\kGuardB}{n}~.
       \end{equation*}
\end{corollary}

\begin{proof}
       This follows from Lemma \ref{lem:oldrule_technical} and Equation \ref{eqn:oldrule-technical-two},
       because we have
       \belowdisplayskip=0pt
       \begin{align*}
                         \ert{C}{0} \cdot \wp{C}{\kGuardB}^n & \eeq 
                         \wp{C}{\ert{C}{0}} \cdot \wp{C}{\kGuardB}^n
                         \tag{by Equation \ref{eqn:oldrule-technical-two}} \\
        &\eeq    \wpFold{C}{\wp{C}{\ert{C}{0}}}{\kGuardB}{n}   
                         \tag{by Lemma \ref{lem:oldrule_technical}} \\
        &\eeq    \wpFold{C}{\ert{C}{0}}{\kGuardB}{n} ~.
        \tag{by Equation \ref{eqn:oldrule-technical-two}}
       \end{align*}
       \normalsize
\end{proof}

With that corollary at hand, we can establish the following lower and upper $\omega$--invariant.
\begin{lemma}[$\omega$--Invariant for universally i.i.d.\ Loops]
       \label{lem:oldrule-omega-invariant}
       Let $C \in \pgcl$ and $\kGuard$ be a guard such that the loop $\WHILEDO{\kGuard}{C}$ is
       universally independent and identically distributed. Furthermore assume 
       \begin{equation}
       \label{eqn:oldrule-omega-condition-one}
       \wp{C}{\ert{C}{0}} = \ert{C}{0} \tag{\ref{eqn:oldrule-technical-two}}
       \end{equation}
       and
       \begin{equation}
       \label{eqn:oldrule-omega-condition-two}
       \wp{C}{1} = 1~.
       \end{equation} 
       Then the following is both an upper and a lower $\omega$-invariant of
       $\WHILEDO{\kGuard}{C}$ with respect to postruntime 0:
       \begin{equation*}
              I_n = 1 + \kGuardB \cdot \left( \ert{C}{0} \cdot
              \sum\limits_{i=0}^{n} \wp{C}{\kGuardB}^i ~+~ 
              \sum\limits_{i=0}^{n-1} \wp{C}{\kGuardB}^i \right)
       \end{equation*} 
\end{lemma}
\begin{proof}
       The $\ertsymbol$--characteristic functional of $\WHILEDO{\kGuard}{C}$ with respect to to postruntime $0$ is given by
       \begin{align*}
		F_0(X) \eeq 1 + \iverson{\neg \varphi} \cdot 0 +  \iverson{\varphi} \cdot \ert{C}{X} \eeq 1 +  \iverson{\varphi} \cdot \ert{C}{X}~.
       \end{align*}
       In order to verify $I_n$ as both an upper and a lower $\omega$-invariant, we first show $F_0 (0) = I_0$. We have 
       \begin{align*}
                              F_0 (0) &\eeq  1 + \kGuardB \cdot \ert{C}{0} \\
              &\eeq  1 + \kGuardB \cdot \left( \ert{C}{0} \cdot \underbrace{\sum\limits_{i=0}^{0} \wp{C}{\kGuardB}^i}_{{}=1}
                              ~+~ \underbrace{\sum\limits_{i=0}^{-1} \wp{C}{\kGuardB}^i}_{{}=0} \right) \\
              &\eeq  I_0 ~.
       \end{align*}
       We also verify $F_0(I_0) = I_1$:
       \begin{align*}
                             F_0 (I_0) &\eeq  1 + \kGuardB \cdot \ert{C}{I_0} \\
              &\eeq  1 + \kGuardB \cdot \ert{C}{1 + \kGuardB \cdot \ert{C}{0}} \tag{by $I_0 = F_0(0)$} \\
              &\eeq  1+\kGuardB \cdot \left(\ert{C}{0} + \wp{C}{1 + \kGuardB \cdot \ert{C}{0}} \right) 
              \tag{by Theorem~\ref{thm:ert-wp}} \\
              &\eeq  1+ \kGuardB \cdot \left(\ert{C}{0} + \wp{C}{1} + \wp{C}{\kGuardB \cdot \ert{C}{0}} \right)
              \tag{by linearity, see Theorem~\ref{thm:basic-prop} (\ref{thm:basic-prop-linearity})} \\
              &\eeq  1+ \kGuardB \cdot \left(\ert{C}{0} + 1 + \wp{C}{\kGuardB \cdot \ert{C}{0}} \right)
              \tag{by Equation \ref{eqn:oldrule-omega-condition-two}} \\
              &\eeq  1+ \kGuardB \cdot \left(\ert{C}{0} + 1 + \wp{C}{\kGuardB} \cdot \ert{C}{0} \right)
              \tag{by Corollary~\ref{cor:oldrule-technical-two} with $n=1$} \\
              &\eeq  1 + \kGuardB \cdot \left( \ert{C}{0} \cdot \sum\limits_{i=0}^{1} \wp{C}{\kGuardB}^i
                              ~+~ \underbrace{\sum\limits_{i=0}^{0} \wp{C}{\kGuardB}^i}_{{}=1} \right) \\
              &\eeq  I_1~.              
       \end{align*}
       Before we show that $F(I_n) = I_{n+1}$ holds, observe the following equations:
       \begin{align}
                         & \wp{C}{\kGuardB \cdot \ert{C}{0} \cdot \sum\limits_{i=0}^{n} \wp{C}{\kGuardB}^i}
                             \notag \\
             & \eeq \sum\limits_{i=0}^{n} \wp{C}{\kGuardB \cdot \ert{C}{0} \cdot \wp{C}{\kGuardB}^i}
             \tag{by linearity, see Theorem~\ref{thm:basic-prop} (\ref{thm:basic-prop-linearity})} \\
             & \eeq \sum\limits_{i=0}^{n} \wp{C}{\kGuardB \cdot \wpFold{C}{\ert{C}{0}}{\kGuardB}{i}}
             \tag{by Corollary \ref{cor:oldrule-technical-two}} \\
             & \eeq \sum\limits_{i=0}^{n} \wp{C}{\kGuardB} \cdot \wpFold{C}{\ert{C}{0}}{\kGuardB}{i}
             \tag{by universal i.i.d.--ness, see Definition \ref{def:iid}} \\
             & \eeq  \sum\limits_{i=0}^{n} \wp{C}{\kGuardB} \cdot \ert{C}{0} \cdot \wp{C}{\kGuardB}^i
             \tag{by Corollary \ref{cor:oldrule-technical-two}} \\
             & \eeq \ert{C}{0} \cdot \sum\limits_{i=i}^{n+1} \wp{C}{\kGuardB}^i
             \label{eqn:oldrule-omega-equation-one}
       \end{align}
       Moreover,
       \begin{align}
                         & \wp{C}{\kGuardB \cdot \sum\limits_{i=0}^{n-1} \wp{C}{\kGuardB}^i} 
                             \notag \\
             & \eeq \sum\limits_{i=0}^{n-1} \wp{C}{\kGuardB \cdot \wp{C}{\kGuardB}^i} 
                            \tag{by linearity, see Theorem~\ref{thm:basic-prop} (\ref{thm:basic-prop-linearity})} \\  
             & \eeq \sum\limits_{i=0}^{n-1} \wp{C}{\kGuardB} \cdot \wp{C}{\kGuardB}^i 
                            \tag{by Lemma \ref{lem:oldrule-technical-three}} \\
             & \eeq \sum\limits_{i=1}^{n} \wp{C}{\kGuardB}^i ~.
                            \label{eqn:oldrule-omega-equation-two}                               
       \end{align}
       We are now in a position two show that $F_0 (I_n) = I_{n+1}$ holds. We have
       \begin{align*}
                            & F_0(I_n) \\
                            &{}={}~  1 + \kGuardB \cdot \ert{C}{I_n} \\
             &{}={}~  1 + \kGuardB \cdot \left(\ert{C}{0} + \wp{C}{I_n} \right) 
                            \tag{by Theorem~\ref{thm:ert-wp}} \\
             &{}={}~  1 + \kGuardB \cdot \left(\ert{C}{0} \right. \\
             &\qquad \left. {}+      \wp{C}{1 + \kGuardB \cdot \left( \ert{C}{0} \cdot
                                         \sum\limits_{i=0}^{n} \wp{C}{\kGuardB}^i ~+~ 
                                         \sum\limits_{i=0}^{n-1} \wp{C}{\kGuardB}^i \right)} \right) \\
             &{}={}~  1 + \kGuardB \cdot \left(\ert{C}{0} \right.  \\    
             &\qquad {}+   \left.     \wp{C}{1 + \kGuardB \cdot  \ert{C}{0} \cdot
                                         \sum\limits_{i=0}^{n} \wp{C}{\kGuardB}^i ~+~ 
                                          \kGuardB \cdot \sum\limits_{i=0}^{n-1} \wp{C}{\kGuardB}^i} \right) \\
              &{}={}~  1 + \kGuardB \cdot \left( \ert{C}{0} + \wp{C}{1} +
                                   \wp{C}{\kGuardB \cdot \ert{C}{0}
                                                \cdot \sum\limits_{i=0}^{n} \wp{C}{\kGuardB}^i} \right. \\
              &\left. \quad \quad \quad \quad \quad \quad 
                                {}+ \wp{C}{\kGuardB \cdot \sum\limits_{i=0}^{n-1} \wp{C}{\kGuardB}^i} \right)                           
                         \tag{by linearity, see Theorem~\ref{thm:basic-prop} (\ref{thm:basic-prop-linearity})} \\
              &{}={}~  1 + \kGuardB \cdot \left( \ert{C}{0} + 1 +
                                   \wp{C}{\kGuardB \cdot \ert{C}{0}
                                                \cdot \sum\limits_{i=0}^{n} \wp{C}{\kGuardB}^i} \right. \\
              &\left. \quad \quad \quad \quad \quad \quad 
                                {}+ \wp{C}{\kGuardB \cdot \sum\limits_{i=0}^{n-1} \wp{C}{\kGuardB}^i} \right)                           
                         \tag{by Equation \ref{eqn:oldrule-omega-condition-two}} \\   
              &{}={}~  1 + \kGuardB \cdot \left( \ert{C}{0} + 1 +
                                   \ert{C}{0} \cdot \sum\limits_{i=1}^{n+1} \wp{C}{\kGuardB}^i \right. \\
              &\left. \quad \quad \quad \quad \quad \quad 
                                {}+ \wp{C}{\kGuardB \cdot \sum\limits_{i=0}^{n-1} \wp{C}{\kGuardB}^i} \right)                           
                         \tag{by Equation \ref{eqn:oldrule-omega-equation-one}} \\         
              &{}={}~  1 + \kGuardB \cdot \left( \ert{C}{0} + 1 +
                                   \ert{C}{0} \cdot \sum\limits_{i=1}^{n+1} \wp{C}{\kGuardB}^i \right. \\
              &\left. \quad \quad \quad \quad \quad \quad 
                                {}+ \sum\limits_{i=1}^{n} \wp{C}{\kGuardB}^i \right)                           
                         \tag{by Equation \ref{eqn:oldrule-omega-equation-two}} \\
               &{}={}~  1 + \kGuardB \cdot \left( \ert{C}{0} \cdot
              \sum\limits_{i=0}^{n+1} \wp{C}{\kGuardB}^i ~+~ 
              \sum\limits_{i=0}^{n} \wp{C}{\kGuardB}^i \right)  \\
              &{}={}~  I_{n+1} ~.      \tag*{\qed}
       \end{align*}
\end{proof}
\noindent
Finally, we are in a position to prove Theorem~\ref{thm:oldrule-proof-rule}.

\begin{proof}
       We show for every state $\sigma \in \States$ that
       \begin{align*}
              & \ert{\WHILEDO{\kGuard}{C}}{f}(\sigma) \eeq 1 + \frac{\kGuardB (\sigma) \cdot \left(1 + \ert{C}{\nkGuardB \cdot f} (\sigma) \right)}{1- \wp{C}{\kGuardB} (\sigma)}  + \nkGuardB (\sigma) \cdot f (\sigma)~.
        \end{align*}
        We distinguish two cases for the probability of the loop guard being true after one execution of the loop body:
        %We now consider the cases 
        $\wp{C}{\kGuardB}(\sigma)<1$
        and $\wp{C}{\kGuardB}(\sigma)=1$. 
        \paragraph{Case $\wp{C}{\kGuardB}(\sigma)<1$:} 
        %Theorem~\ref{thm:omega-invariants}, Equation~\ref{eqn:oldrule-proof-rule-omega-invariant},
        %and the closed form of the geometric series yield
        %
        %
        \begin{align}
                         & \ert{\WHILEDO{\kGuard}{C}}{0} (\sigma) \notag \\
                {}={}~& \lim_{n\to\infty} ~ \left( 1 + \kGuardB (\sigma) \cdot \left( \ert{C}{0} (\sigma) \cdot
                             \sum\limits_{i=0}^{n} \wp{C}{\kGuardB} (\sigma)^i ~+~ 
                             \sum\limits_{i=0}^{n-1} \wp{C}{\kGuardB} (\sigma)^i \right) \right) 
                             \tag{by Theorem~\ref{thm:omega-invariants} and  Lemma~\ref{lem:oldrule-omega-invariant}} \\
                {}={}~& 1 + \kGuardB (\sigma) \cdot \left( \ert{C}{0} (\sigma) \cdot
                             \sum\limits_{i=0}^{\infty} \wp{C}{\kGuardB} (\sigma)^i ~+~ 
                             \sum\limits_{i=0}^{\infty} \wp{C}{\kGuardB} (\sigma)^i \right) 
                             \notag \\
                 {}={}~& 1 + \kGuardB (\sigma) \cdot \left( 
                               \frac{\ert{C}{0} (\sigma)}{1-\wp{C}{\kGuardB} (\sigma)} + 
                                \frac{1}{1-\wp{C}{\kGuardB} (\sigma)} \right)      
                                \tag{geometric series} \\
                 {}={}~& 1 + \frac{\kGuardB (\sigma) \cdot \left( 
                               \ert{C}{0} (\sigma) + 1 \right)}{1-\wp{C}{\kGuardB} (\sigma)}~. 
                               \label{eqn:oldrule-proof-caseone-appendix}                                                                    
        \end{align}
        Now, by Theorem~\ref{thm:ert-wp}, Theorem~\ref{thm:oldrule-wpsemantics}~(\ref{thm:oldrule-wpsemantics-one}), and Equation~\ref{eqn:oldrule-proof-caseone-appendix}, we obtain
        \begin{align*}
                         & \ert{\WHILEDO{\kGuard}{C}}{f} (\sigma) \\
               {}={}~& \ert{\WHILEDO{\kGuard}{C}}{0} (\sigma) + \wp{\WHILEDO{\kGuard}{C}}{f} (\sigma)   
                            \tag{by Theorem~\ref{thm:ert-wp}} \\
               {}={}~& 1 + \frac{\kGuardB (\sigma) \cdot \left( 
                            \ert{C}{0} (\sigma) + 1 \right)}{1-\wp{C}{\kGuardB} (\sigma)} +
                            \iverson{\kGuard}(\sigma) \cdot 
                            \frac{\wp{C}{\iverson{\neg \kGuard} \cdot f}(\sigma)}{1-\wp{C}{\iverson{\kGuard}}(\sigma)}  + \iverson{\neg \kGuard}(\sigma) \cdot f(\sigma)
                            \tag{by Theorem~\ref{thm:oldrule-wpsemantics}~(\ref{thm:oldrule-wpsemantics-one}) and Equation~\ref{eqn:oldrule-proof-caseone-appendix}} \\
               {}={}~& 1 + \frac{\kGuardB (\sigma) \cdot \left( 1 + \ert{C}{0} (\sigma)
                            + \wp{C}{\nkGuardB \cdot f} (\sigma) \right)}{1- \wp{C}{\kGuardB} (\sigma)} 
                             + \nkGuardB (\sigma) \cdot f (\sigma)\\
               {}={}~& 1 + \frac{\kGuardB (\sigma) \cdot \left( 1 + \ert{C}{\nkGuardB \cdot f} (\sigma) \right)}{1- \wp{C}{\kGuardB} (\sigma)}  + \nkGuardB (\sigma) \cdot f (\sigma)~. \tag{by Theorem~\ref{thm:ert-wp}}                                  
        \end{align*}
        \emph{Case $\wp{C}{\kGuardB} (\sigma)=1$:} We distinguish the cases $\kGuardB (\sigma) =0$ and $\kGuardB (\sigma)=1$.
        First suppose $\kGuardB (\sigma) =0$. Then from Theorem~\ref{thm:omega-invariants} and Lemma~\ref{lem:oldrule-omega-invariant} it follows that
        \begin{align}
               & \ert{\WHILEDO{\kGuard}{C}}{0} (\sigma) \notag \\
               &{}={}~ \lim_{n\to\infty} ~ \left( 1 + \underbrace{\kGuardB (\sigma)}_{{}={}0} \cdot \left( \ert{C}{0} (\sigma) \cdot
                             \sum\limits_{i=0}^{n} \wp{C}{\kGuardB} (\sigma)^i ~+~ 
                             \sum\limits_{i=0}^{n-1} \wp{C}{\kGuardB} (\sigma)^i \right) \right) 
                             \tag{by Theorem~\ref{thm:omega-invariants} and  Lemma~\ref{lem:oldrule-omega-invariant}} \\
               &{}={}~ \lim_{n\to\infty} ~1 \eeq  1~. \label{eqn:oldrule-proof-casetwo-one-appendix}            
        \end{align}
        Theorem~\ref{thm:oldrule-wpsemantics}~(\ref{thm:oldrule-wpsemantics-two}) and Equation~\ref{eqn:oldrule-proof-casetwo-one-appendix} now yield
        \begin{align*}
                         & \ert{\WHILEDO{\kGuard}{C}}{f} (\sigma) \\
               &{}={}~ \ert{\WHILEDO{\kGuard}{C}}{0} (\sigma) + \wp{\WHILEDO{\kGuard}{C}}{f} (\sigma)     
                            \tag{by Theorem~\ref{thm:ert-wp}} \\
               &{}={}~ 1 + \nkGuardB (\sigma) \cdot f (\sigma)
                            \tag{by Theorem~\ref{thm:oldrule-wpsemantics}~(\ref{thm:oldrule-wpsemantics-two}) and Equation~\ref{eqn:oldrule-proof-casetwo-one-appendix}} \\
               &{}={}~  1 + \underbrace{\frac{\kGuardB (\sigma) \cdot \left(1+\ert{C}{\nkGuardB \cdot f} \right)}{1- \wp{C}{\kGuardB} (\sigma)}}_{{}={}\frac{0}{0} \coloneq 0} 
                              + \nkGuardB (\sigma) \cdot f (\sigma)~.            
        \end{align*}
        To prove the remaining case, suppose $\kGuardB (\sigma)=1$. Theorem~\ref{thm:omega-invariants} and Lemma~\ref{lem:oldrule-omega-invariant} then imply
        \begin{align}
                         & \ert{\WHILEDO{\kGuard}{C}}{0} (\sigma) \notag \\
                &{}={}~ \lim_{n\to\infty} ~ \left( 1 + \underbrace{\kGuardB (\sigma)}_{{}=1} \cdot \left( \ert{C}{0} (\sigma) \cdot
                             \sum\limits_{i=0}^{n} \underbrace{\wp{C}{\kGuardB} (\sigma)^i}_{{}={}1} ~+~ 
                             \sum\limits_{i=0}^{n-1} \underbrace{\wp{C}{\kGuardB} (\sigma)^i}_{{}={}1} \right) \right) 
                             \tag{by Theorem~\ref{thm:omega-invariants} and  Lemma~\ref{lem:oldrule-omega-invariant}} \\
                &{}={}~ \lim_{n\to\infty} ~ 1 + \ert{C}{0} (\sigma) \cdot \sum\limits_{i=0}^{n} 1 ~+~\sum\limits_{i=0}^{n-1} 1
                             \notag \\
                &{}={}~ \lim_{n\to\infty} ~ 1 + \ert{C}{0} (\sigma) \cdot (n+1) +n 
                             \notag \\
                &{}={}~ \infty~. \label{eqn:oldrule-proof-casetwo-two-appendix}  
        \end{align}
       Using Theorem~\ref{thm:ert-wp} and Equation~\ref{eqn:oldrule-proof-casetwo-two-appendix}, we obtain
       \begin{align*}
                        & \ert{\WHILEDO{\kGuard}{C}}{f} (\sigma) \\
               &{}={}~ \ert{\WHILEDO{\kGuard}{C}}{0} (\sigma) + \wp{\WHILEDO{\kGuard}{C}}{f} (\sigma)     
                            \tag{by Theorem~\ref{thm:ert-wp}} \\
               &{}={}~ \infty + \nkGuardB (\sigma) \cdot f (\sigma)
                            \tag{by Equation~\ref{eqn:oldrule-proof-casetwo-two-appendix} and Theorem~\ref{thm:oldrule-wpsemantics}(\ref{thm:oldrule-wpsemantics-two})} \\
               &{}={}~ \infty \\
               &{}={}~ 1 + \underbrace{\frac{\kGuardB (\sigma) \cdot \left( 1+ \ert{C}{\nkGuardB \cdot f}(\sigma) \right)}{1- \wp{C}{\kGuardB} (\sigma)}}_{{}={}\frac{1}{0} {}\coloneq{}~ \infty} 
 + \nkGuardB (\sigma) \cdot f (\sigma)~.  \tag*{\qed}
       \end{align*}
\end{proof}

\subsection{Proof of Lemma~\ref{lem:newrule-main}}
\label{proof-lem:newrule-main}
\begin{proof}
       By induction on the structure of C. As the induction base we have the atomic programs: \\ \\
       \emph{$\SKIP$:} We have
       \begin{equation*}
              \wp{\SKIP}{g \cdot f} \eeq  g \cdot f \eeq  g \cdot \wp{\SKIP}{f}~. 
              \tag{by Table~\ref{table:wp}}
       \end{equation*} \\
       \emph{$\EMPTY$:} Analogous to $\SKIP$. \\ \\
       \emph{$\DIVERGE$:} We have
       \begin{equation*}
              \wp{\DIVERGE}{g \cdot f} \eeq  0 \eeq  g \cdot \wp{\DIVERGE}{f}~.
              \tag{by Table~\ref{table:wp}}
       \end{equation*}
       \emph{$\PASSIGN{x}{\mu}$:} We have
       \begin{align*}
                            \wp{\PASSIGN{x}{\mu}}{g \cdot f} \eeq & \lambda \sigma\mydot \Exp{\Rats}{\big(\lambda v\mydot (f \cdot g)\subst{x}{v}\big)}{\mu_\sigma} 
                            \tag{by Table~\ref{table:wp}}\\
             \eeq & \lambda \sigma\mydot \Exp{\Rats}{\big(\lambda v\mydot f\subst{x}{v}\big) \cdot g}{\mu_\sigma} 
                            \tag{$\RelNewRule{g}{(\PASSIGN{x}{\mu})}$ by assumption} \\
             \eeq & g \cdot \left( \lambda \sigma\mydot \Exp{\Rats}{\big(\lambda v\mydot f\subst{x}{v}\big)}{\mu_\sigma} \right) \\
             \eeq & g \cdot \wp{\PASSIGN{x}{\mu}}{f}~.
       \end{align*}
       As the induction hypothesis we now assume that for arbitrary but fixed $C_1, C_2 \in \pgcl$ and all $f,g \in E$ 
       with $\RelNewRule{g}{C_1}$ and $\RelNewRule{g}{C_2}$ it holds that both
       \begin{equation*}
              \wp{C_1}{g \cdot f} \eeq  g \cdot \wp{C_1}{f}
       \end{equation*}
       and
       \begin{equation*}
              \wp{C_2}{g \cdot f} \eeq  g \cdot \wp{C_2}{f}~.
       \end{equation*}  \\     
       \emph{$\ITE{\kGuard}{C_1}{C_2}$:} We have
       \begin{align*}
                        & \wp{\ITE{\kGuard}{C_1}{C_2}}{g \cdot f} \\
              {}={}~& \kGuardB \cdot \wp{C_1}{g \cdot f} + \nkGuardB \cdot \wp{C_2}{g \cdot f}
                           \tag{by Table~\ref{table:wp}} \\
              {}={}~& \kGuardB \cdot g \cdot \wp{C_1}{f} + \nkGuardB \cdot \wp{C_2}{g \cdot f} 
                           \tag{$\RelNewRule{g}{C_1}$ and I.H.\ on $C_1$} \\
              {}={}~&  \kGuardB \cdot g \cdot \wp{C_1}{f} + \nkGuardB \cdot g \cdot  \wp{C_2}{f} 
                           \tag{$\RelNewRule{g}{C_2}$ and I.H.\ on $C_2$} \\
              {}={}~& g \cdot \left(  \kGuardB \cdot \wp{C_1}{f} + \nkGuardB \cdot  \wp{C_2}{f} \right) \\
              {}={}~& g \cdot \wp{\ITE{\kGuard}{C_1}{C_2}}{f}~.
                           \tag{by Table~\ref{table:wp}}
       \end{align*}
       \\       
        \emph{$\COMPOSE{C_1}{C_2}$: } We have
        \begin{align*}
                               \wp{\COMPOSE{C_1}{C_2}}{g \cdot f}
                \eeq & \wp{C_1}{\wp{C_2}{g \cdot f}}
                               \tag{by Table~\ref{table:wp}} \\
                \eeq & \wp{C_1}{g \cdot \wp{C_2}{f}}
                               \tag{$\RelNewRule{g}{C_2}$ and I.H.\ on $C_2$} \\
                \eeq & g \cdot \wp{C_1}{\wp{C_2}{f}}
                               \tag{$\RelNewRule{g}{C_1}$ and I.H.\ on $C_1$} \\
                \eeq & g \cdot \wp{\COMPOSE{C_1}{C_2}}{f} ~.
                               \tag{by Table~\ref{table:wp}}
        \end{align*} \\
        \emph{$\WHILEDO{\kGuard}{C_1}$:} This case is more involved. Recall that
        \begin{equation}
               \label{eqn:newrule:lemmavars_sup}
               \wp{\WHILEDO{\kGuard}{C_1}}{h} \eeq  \sup_{n\in \Nats}~ \wp{\WHILEDOapprox{\kGuard}{C_1}{n}}{h}
        \end{equation}
        holds for all $h \in \E$. Thus we show 
        \begin{equation}
               \label{eqn:newrule-lemmavars-while}
               \wp{\WHILEDOapprox{\kGuard}{C_1}{n}}{g \cdot f} \eeq  g \cdot \wp{\WHILEDOapprox{\kGuard}{C_1}{n}}{f}
        \end{equation}
        for all $n \in \Nats$, which implies the desired result. We proceed by induction on $n$. \\ \\
        \emph{Induction base $n=0$.} We have 
        \begin{align*}
                              &\wp{\WHILEDOapprox{\kGuard}{C_1}{0}}{g \cdot f} \\
                              &{}={}~  \wp{\DIVERGE}{g \cdot f}
                              \tag{by Definition~\ref{def:finite_approximations}} \\
                              &{}={}~ 0
                              \tag{by Table~\ref{table:wp}} \\
                              &{}={}~ g \cdot 0 \\
                              &{}={}~  g \cdot \wp{\WHILEDOapprox{\kGuard}{C_1}{0}}{ f}~.
                              \tag{by Definition~\ref{def:finite_approximations}}
        \end{align*} \\
        \emph{Induction Hypothesis.} Assume that Equation~\ref{eqn:newrule-lemmavars-while} holds for some arbitrary but fixed $n \in \Nats$. \\ \\
        \emph{Induction Step $n \mapsto n+1$.} We have
        \begin{align*}
                          & \wp{\WHILEDOapprox{\kGuard}{C_1}{n+1}}{g \cdot f} \\
              &{}={}~  \wp{\ITE{\kGuard}{\COMPOSE{C_1}{\WHILEDOapprox{\kGuard}{C_1}{n}}}{\SKIP}}{g \cdot f}
                             \tag{by Definition~\ref{def:finite_approximations}} \\
              &{}={}~ \kGuardB \cdot  \wp{C_1}{\wp{\WHILEDOapprox{\kGuard}{C_1}{n}}{g \cdot f}} + \nkGuardB \cdot g \cdot f
                             \tag{by Table~\ref{table:wp}} \\
              &{}={}~ \kGuardB \cdot \wp{C_1}{g \cdot \wp{\WHILEDOapprox{\kGuard}{C_1}{n}}{f}} + \nkGuardB \cdot g \cdot f     
                             \tag{I.H.\ on $n$}  \\
              &{}={}~ \kGuardB \cdot g \cdot \wp{C_1}{\wp{\WHILEDOapprox{\kGuard}{C_1}{n}}{f}} + \nkGuardB \cdot g \cdot f   
                             \tag{$\RelNewRule{g}{C_1}$ and I.H.\ on $C_1$} \\
              &{}={}~ g \cdot \left(  \kGuardB \cdot \wp{C_1}{\wp{\WHILEDOapprox{\kGuard}{C_1}{n}}{f}} + \nkGuardB \cdot f   \right) \\
              &{}={}~ g \cdot \wp{\ITE{\kGuard}{\COMPOSE{C_1}{\WHILEDOapprox{\kGuard}{C_1}{n}}}{\SKIP}}{f} 
                                \tag{by Table~\ref{table:wp}} \\
              &{}={}~ g \cdot \wp{\WHILEDOapprox{\kGuard}{C_1}{n+1}}{f}~.
                             \tag{by Definition~\ref{def:finite_approximations}}
        \end{align*}
        Overall, we get
        \begin{align*}
                              \wp{\WHILEDO{\kGuard}{C_1}}{g \cdot f} &\eeq  \sup_{n\in \Nats}~ \wp{\WHILEDOapprox{\kGuard}{C_1}{n}}{g \cdot f} 
                              \tag{by Equation~\ref{eqn:newrule:lemmavars_sup}} \\
               &\eeq  \sup_{n\in \Nats}~ g \cdot \wp{\WHILEDOapprox{\kGuard}{C_1}{n}}{f} 
                              \tag{by Equation~\ref{eqn:newrule-lemmavars-while}} \\
               &\eeq  g \cdot ~ \sup_{n\in \Nats}~ \wp{\WHILEDOapprox{\kGuard}{C_1}{n}}{f} \\
               &\eeq  g \cdot \wp{\WHILEDO{\kGuard}{C_1}}{f}~.
                              \tag{by Equation~\ref{eqn:newrule:lemmavars_sup}}
        \end{align*} \\
        \emph{$\REPEATUNTIL{\kGuard}{C_1}$:} We have
        \begin{align*}
                              \wp{\REPEATUNTIL{C_1}{\kGuard}}{g \cdot f} &\eeq  \wp{\COMPOSE{C_1}{\WHILEDO{\kGuard}{C_1}}}{g\cdot f} \\
               &\eeq  \wp{C_1}{\wp{\WHILEDO{\kGuard}{C_1}}{g\cdot f}} 
                              \tag{by Table~\ref{table:wp}} \\
               &\eeq  \wp{C_1}{g \cdot \wp{\WHILEDO{\kGuard}{C_1}}{f}}           
                              \tag{see case $\WHILEDO{\kGuard}{C_1}$} \\
               &\eeq  g \cdot \wp{C_1}{\wp{\WHILEDO{\kGuard}{C_1}}{f}} 
                              \tag{$\RelNewRule{g}{C_1}$ and I.H.\ on $C_1$} \\
               &\eeq  g \cdot \wp{\REPEATUNTIL{C_1}{\kGuard}}{f}
                              \tag{by Table~\ref{table:wp}}~.                           
        \end{align*}
\end{proof}
\noindent
%
%
%
%
%\subsection{Characterization of the $\wpsymbol$--Semantics of an $f$--i.i.d.\ Loop's Finite Approximations}
\subsection{Proof of Lemma~\ref{thm:newrule_wp_finite_approximations}}
\label{lem:newrule_wp_finite_approximations}

\begin{proof}
       By induction on $n$. We consider the cases $n=1$ and $n=2$ as the induction base.
       For $n=1$, we have
       \begin{align}
              \wp{\WHILEDOapprox{\kGuard}{C}{1}}{f} &\eeq 
              \wp{\ITE{\kGuard}{\COMPOSE{C}{\WHILEDOapprox{\kGuard}{C}{0}}}{\SKIP}}{f}
              \tag{by Definition~\ref{def:finite_approximations}} \\
              &\eeq  \wp{\ITE{\kGuard}{\COMPOSE{C}{\DIVERGE}}{\SKIP}}{f} \tag{by Definition~\ref{def:finite_approximations}} \\
              &\eeq  \iverson{\kGuard} \cdot \wp{C}{0} + \iverson{\neg \kGuard} \cdot f \tag{by \autoref{table:wp}} \\
              &\eeq  \iverson{\kGuard} \cdot 0 + \iverson{\neg \kGuard} \cdot f \tag{by linearity, see Theorem~\ref{thm:basic-prop} (\ref{thm:basic-prop-linearity})} \\
              &\eeq  \iverson{\neg \kGuard} \cdot f \label{eqn:newrule-while-one} \\
              &\eeq  \iverson{\kGuard} \cdot 0 + \iverson{\neg \kGuard} \cdot f \notag \\
              &\eeq  \iverson{\kGuard} \cdot \left( \wp{C}{\iverson{\neg \kGuard} \cdot f}
               \cdot \sum\limits_{i=0}^{-1} \wp{C}{\iverson{\kGuard}}^i \right) + \iverson{\neg \kGuard} \cdot f~. 
               \notag
       \end{align}
       For $n=2$, we have
       \begin{align*}
        \wp{\WHILEDOapprox{\kGuard}{C}{2}}{f} &\eeq 
              \wp{\ITE{\kGuard}{\COMPOSE{C}{\WHILEDOapprox{\kGuard}{C}{1}}}{\SKIP}}{f}
              \tag{by Definition~\ref{def:finite_approximations}} \\
              &\eeq  \iverson{\kGuard} \cdot \wp{C}{\wp{\WHILEDOapprox{\kGuard}{C}{1}}{f}} + \iverson{\neg \kGuard} + f  \tag{by \autoref{table:wp}} \\
              &\eeq  \iverson{\kGuard} \cdot \wp{C}{\iverson{\neg \kGuard} \cdot f} + \iverson{\neg \kGuard} \cdot f
              \tag{by \autoref{eqn:newrule-while-one}} \\
              &\eeq  \iverson{\kGuard} \cdot \left(  \wp{C}{\iverson{\neg \kGuard} \cdot f}
               \cdot \sum\limits_{i=0}^{0} \wp{C}{\iverson{\kGuard}}^i \right) + \iverson{\neg \kGuard} \cdot f~.
       \end{align*}
       Before we perform the inductive step, observe the following equation implied by 
       Lemma~\ref{lem:newrule-main},
       which holds for all $n \in \Nats$:
       \begin{align}
                        &\wp{C}{\iverson{\kGuard} \cdot \wp{C}{\iverson{\neg \kGuard} \cdot f}
                           \cdot \sum\limits_{i=0}^{n-2} \wp{C}{\iverson{\kGuard}}^i} \notag \\
              &{}={}~ \sum\limits_{i=0}^{n-2} \wp{C}{\iverson{\kGuard} \cdot \wp{C}{\iverson{\neg \kGuard} \cdot f}
                           \cdot \wp{C}{\iverson{\kGuard}}^i} 
                           \tag{by linearity, see Theorem~\ref{thm:basic-prop} (\ref{thm:basic-prop-linearity})} \\
              &{}={}~ \sum\limits_{i=0}^{n-2} \wp{C}{\iverson{\kGuard} \cdot \wp{C}{\iverson{\neg \kGuard} \cdot f}}
                           \cdot \wp{C}{\iverson{\kGuard}}^i
                           \tag{by Lemma~\ref{lem:newrule-main}, $\RelNewRule{\wp{C}{\iverson{\kGuard}}}{C}$}  \\
              &{}={}~ \sum\limits_{i=0}^{n-2} \wp{C}{\iverson{\kGuard}} \cdot \wp{C}{\iverson{\neg \kGuard} \cdot f}
                           \cdot \wp{C}{\iverson{\kGuard}}^i
                           \tag{by Lemma~\ref{lem:newrule-main}, $\RelNewRule{\wp{C}{\iverson{\neg \kGuard} \cdot f}}{C}$}  \\
              &{}={}~ \wp{C}{\iverson{\kGuard}} \cdot \wp{C}{\iverson{\neg \kGuard} \cdot f}
       \cdot \sum\limits_{i=0}^{n-2}  \wp{C}{\iverson{\kGuard}}^i \label{eqn: newrule-semantics-proof}
       \end{align}
       We now assume the lemma holds for some arbitrary but fixed $n \in \Nats \setminus \{ 0 \}$. 
       We compute
       \begin{align*}
       &\wp{\WHILEDOapprox{\kGuard}{C}{n+1}}{f} \\
       &{}={}~ \wp{\ITE{\kGuard}{\COMPOSE{C}{\WHILEDOapprox{\kGuard}{C}{n}}}{\SKIP}}{f}
                    \tag{By Definition \ref{def:finite_approximations}} \\
       &{}={}~ \iverson{\kGuard} \cdot \wp{C}{\wp{\WHILEDOapprox{\kGuard}{C}{n}}{f}} 
                    + \iverson{\neg \kGuard} \cdot f \\
       &{}={}~ \iverson{\kGuard} \cdot \wp{C}{ \iverson{\kGuard} \cdot \wp{C}{\iverson{\neg \kGuard} \cdot f}
                    \cdot \sum\limits_{i=0}^{n-2} \wp{C}{\iverson{\kGuard}}^i + \iverson{\neg \kGuard} \cdot f}
                    + \iverson{\neg \kGuard} \cdot f
       \tag{by I.H.} \\
       &{}={}~ \iverson{\kGuard} \cdot \left( \wp{C}{\iverson{\kGuard} \cdot \wp{C}{\iverson{\neg \kGuard} \cdot f}
                    \cdot \sum\limits_{i=0}^{n-2} \wp{C}{\iverson{\kGuard}}^i}
                    + \wp{C}{\iverson{\neg \kGuard} \cdot f} \right) + \iverson{\neg \kGuard} \cdot f
                    \tag{by linearity, see Theorem~\ref{thm:basic-prop} (\ref{thm:basic-prop-linearity})} \\
       &{}={}~  \iverson{\kGuard} \cdot \left( \wp{C}{\iverson{\kGuard}} \cdot \wp{C}{\iverson{\neg \kGuard} \cdot f}
                     \cdot \sum\limits_{i=0}^{n-2} \left(  \wp{C}{\iverson{\kGuard}}^i \right)
                  + \wp{C}{\iverson{\neg \kGuard} \cdot f} \right) + \iverson{\neg \kGuard} \cdot f
                     \tag{By Equation \ref{eqn: newrule-semantics-proof}} \\
       &{}={}~  \iverson{\kGuard} \cdot \left(\wp{C}{\iverson{\neg \kGuard} \cdot f}
                     \cdot \sum\limits_{i=1}^{n-1} \left(  \wp{C}{\iverson{\kGuard}}^i \right)
                  + \wp{C}{\iverson{\neg \kGuard} \cdot f} \right) + \iverson{\neg \kGuard} \cdot f \\
       &{}={}~  \iverson{\kGuard} \cdot \left(\wp{C}{\iverson{\neg \kGuard} \cdot f}
                     \cdot \sum\limits_{i=0}^{n-1}  \wp{C}{\iverson{\kGuard}}^i  \right) 
                     + \iverson{\neg \kGuard} \cdot f ~.
       \end{align*}
\end{proof}
\noindent
\subsection{An $\omega$--Invariant for $f$--i.i.d. Loops w.r.t.\ Postruntime $0$}
\label{lem:newrule-omega-invariant}

\begin{lemma}[$\omega$--Invariant for $0$--i.i.d.\ Loops]
       \label{lem:newrule-omega-invariant}
       Let $C \in \pgcl$, $\kGuard$ be a guard, and $f \in \E$ such that the loop $\WHILEDO{\kGuard}{C}$ is $0$--i.i.d. Furthermore, assume 
       \begin{equation}
       \label{eqn:newrule-omega-condition-two}
              \wp{C}{1} = 1
       \end{equation} 
       and
       \begin{equation}
       \label{eqn:newrule-omega-condition-one}
              \RelNewRule{\ert{C}{0}}{C}~.
       \end{equation}
       Then the following is both an upper and a lower $\omega$-invariant of the loop
       $\WHILEDO{\kGuard}{C}$ with respect to postruntime 0:
       \begin{equation*}
              I_n = 1 + \kGuardB \cdot \left( \ert{C}{0} \cdot
              \sum\limits_{i=0}^{n} \wp{C}{\kGuardB}^i ~+~ 
              \sum\limits_{i=0}^{n-1} \wp{C}{\kGuardB}^i \right)
       \end{equation*} 
\end{lemma}
\begin{proof}
       Let $F_0$ denote the characteristic functional of the loop $\WHILEDO{\kGuard}{C}$ with respect to to postruntime $0$.
       In order to verify $I_n$ as both an upper and a lower $\omega$-invariant, we first show $F_0 (0) = I_0$. We have 
       \begin{align*}
                              F_0 (0) &\eeq  1 + \kGuardB \cdot \ert{C}{0} \\
              &\eeq  1 + \kGuardB \cdot \left( \ert{C}{0} \cdot \sum\limits_{i=0}^{0} \wp{C}{\kGuardB}^i
                              ~+~ \sum\limits_{i=0}^{-1} \wp{C}{\kGuardB}^i \right) \\
              &\eeq  I_0 ~.
       \end{align*}
       We also verify $F_0(I_0) = I_1$:
       \begin{align*}
                             F_0 (I_0) &\eeq  1 + \kGuardB \cdot \ert{C}{I_0} \\
              &\eeq  1 + \kGuardB \cdot \ert{C}{1 + \kGuardB \cdot \ert{C}{0}} \\
              &\eeq  1+\kGuardB \cdot \left(\ert{C}{0} + \wp{C}{1 + \kGuardB \cdot \ert{C}{0}} \right)
              \tag{by Theorem~\ref{thm:ert-wp}} \\
              &\eeq  1+ \kGuardB \cdot \left(\ert{C}{0} + \wp{C}{1} + \wp{C}{\kGuardB \cdot \ert{C}{0}} \right)
              \tag{by linearity, see Theorem~\ref{thm:basic-prop} (\ref{thm:basic-prop-linearity})} \\
              &\eeq  1+ \kGuardB \cdot \left(\ert{C}{0} + 1 + \wp{C}{\kGuardB \cdot \ert{C}{0}} \right)
              \tag{by Equation \ref{eqn:newrule-omega-condition-two}} \\
              &\eeq  1+ \kGuardB \cdot \left(\ert{C}{0} + 1 + \wp{C}{\kGuardB} \cdot \ert{C}{0} \right)
              \tag{by Lemma~\ref{lem:newrule-main}, $\RelNewRule{\ert{C}{0}}{C}$} \\
              &\eeq  1 + \kGuardB \cdot \left( \ert{C}{0} \cdot \sum\limits_{i=0}^{1} \wp{C}{\kGuardB}^i
                              ~+~ \sum\limits_{i=0}^{0} \wp{C}{\kGuardB}^i \right) \\
              &\eeq  I_1~.              
       \end{align*}
       Before we turn on showing that $F(I_n) = I_{n+1}$ holds, observe the following equations.
       Lemma~\ref{lem:newrule-main} yields
       \begin{align}
                         & \wp{C}{\kGuardB \cdot \ert{C}{0} \cdot \sum\limits_{i=0}^{n} \wp{C}{\kGuardB}^i}
                             \notag \\
             &{}={}~  \sum\limits_{i=0}^{n} \wp{C}{\kGuardB \cdot \ert{C}{0} \cdot \wp{C}{\kGuardB}^i}
             \tag{by linearity, see Theorem~\ref{thm:basic-prop} (\ref{thm:basic-prop-linearity})} \\
             &{}={}~ \sum\limits_{i=0}^{n} \wp{C}{\kGuardB \cdot \ert{C}{0}} \cdot \wp{C}{\kGuardB}^i
             \tag{by Lemma~\ref{lem:newrule-main}, $\RelNewRule{\wp{C}{\kGuardB}}{C}$} \\
             &{}={}~ \sum\limits_{i=0}^{n} \wp{C}{\kGuardB} \cdot \ert{C}{0} \cdot \wp{C}{\kGuardB}^i
             \tag{by Lemma~\ref{lem:newrule-main}, $\RelNewRule{\ert{C}{0}}{C}$} \\
             &{}={}~ \ert{C}{0} \cdot \sum\limits_{i=i}^{n+1} \wp{C}{\kGuardB}^i~.
             \label{eqn:newrule-omega-equation-one}
       \end{align}
       Lemma \ref{lem:newrule-main} implies further
       \begin{align}
                         & \wp{C}{\kGuardB \cdot \sum\limits_{i=0}^{n-1} \wp{C}{\kGuardB}^i} 
                             \notag \\
             &{}={}~ \sum\limits_{i=0}^{n-1} \wp{C}{\kGuardB \cdot \wp{C}{\kGuardB}^i} 
                            \tag{by linearity, see Theorem~\ref{thm:basic-prop} (\ref{thm:basic-prop-linearity})} \\  
             &{}={}~ \sum\limits_{i=0}^{n-1} \wp{C}{\kGuardB} \cdot \wp{C}{\kGuardB}^i 
                            \tag{by Lemma \ref{lem:newrule-main}, $\RelNewRule{\wp{C}{\kGuardB}}{C}$} \\
             &{}={}~ \sum\limits_{i=1}^{n} \wp{C}{\kGuardB}^i ~.
                            \label{eqn:newrule-omega-equation-two}                               
       \end{align}
       We are now in a position two show that $F_0 (I_n) = I_{n+1}$ holds. We have
       \begin{align*}
                            &F_0(I_n) \\
             &{}={}~  1 + \kGuardB \cdot \ert{C}{I_n} \\
             &{}={}~  1 + \kGuardB \cdot \left(\ert{C}{0} + \wp{C}{I_n} \right) 
                            \tag{by Theorem~\ref{thm:ert-wp}} \\
             &{}={}~  1 + \kGuardB \cdot \left(\ert{C}{0} \right. \\
             &\qquad \left. +     
                             \wp{C}{1 + \kGuardB \cdot \left( \ert{C}{0} \cdot
                                         \sum\limits_{i=0}^{n} \wp{C}{\kGuardB}^i ~+~ 
                                         \sum\limits_{i=0}^{n-1} \wp{C}{\kGuardB}^i \right)} \right) \\
             &{}={}~  1 + \kGuardB \cdot \left(\ert{C}{0} \right. \\ 
             &\qquad \left. + \wp{C}{1 + \kGuardB \cdot  \ert{C}{0} \cdot
                                         \sum\limits_{i=0}^{n} \wp{C}{\kGuardB}^i ~+~ 
                                          \kGuardB \cdot \sum\limits_{i=0}^{n-1} \wp{C}{\kGuardB}^i} \right) \\
              &{}={}~  1 + \kGuardB \cdot \left( \ert{C}{0} + \wp{C}{1} +
                                   \wp{C}{\kGuardB \cdot \ert{C}{0}
                                                \cdot \sum\limits_{i=0}^{n} \wp{C}{\kGuardB}^i} \right. \\
              &\left. \quad \quad \quad \quad \quad \quad 
                                {}+ \wp{C}{\kGuardB \cdot \sum\limits_{i=0}^{n-1} \wp{C}{\kGuardB}^i} \right)                           
                         \tag{by linearity, see Theorem~\ref{thm:basic-prop} (\ref{thm:basic-prop-linearity})} \\
              &{}={}~  1 + \kGuardB \cdot \left( \ert{C}{0} + 1 +
                                   \wp{C}{\kGuardB \cdot \ert{C}{0}
                                                \cdot \sum\limits_{i=0}^{n} \wp{C}{\kGuardB}^i} \right. \\
              &\left. \quad \quad \quad \quad \quad \quad 
                                {}+ \wp{C}{\kGuardB \cdot \sum\limits_{i=0}^{n-1} \wp{C}{\kGuardB}^i} \right)                           
                         \tag{by Equation \ref{eqn:newrule-omega-condition-two}} \\   
              &{}={}~  1 + \kGuardB \cdot \left( \ert{C}{0} + 1 +
                                   \ert{C}{0} \cdot \sum\limits_{i=1}^{n+1} \wp{C}{\kGuardB}^i \right. \\
              &\left. \quad \quad \quad \quad \quad \quad 
                                {}+ \wp{C}{\kGuardB \cdot \sum\limits_{i=0}^{n-1} \wp{C}{\kGuardB}^i} \right)                           
                         \tag{by Equation \ref{eqn:newrule-omega-equation-one}} \\         
              &{}={}~  1 + \kGuardB \cdot \left( \ert{C}{0} + 1 +
                                   \ert{C}{0} \cdot \sum\limits_{i=1}^{n+1} \wp{C}{\kGuardB}^i \right. \\
              &\left. \quad \quad \quad \quad \quad \quad 
                                {}+ \sum\limits_{i=1}^{n} \wp{C}{\kGuardB}^i \right)                           
                         \tag{by Equation \ref{eqn:newrule-omega-equation-two}} \\
               &{}={}~  1 + \kGuardB \cdot \left( \ert{C}{0} \cdot
              \sum\limits_{i=0}^{n+1} \wp{C}{\kGuardB}^i ~+~ 
              \sum\limits_{i=0}^{n} \wp{C}{\kGuardB}^i \right)  \\
              &{}={}~  I_{n+1} ~.      
       \end{align*}
\end{proof}

\subsection{Remaining case of Theorem~\ref{thm:newrule-proof-rule}}
\label{app:newrule-proof-rule}

\begin{proof}
To prove the remaining case, suppose $\kGuardB (\sigma)=1$. Theorem~\ref{thm:omega-invariants} and Lemma~\ref{lem:newrule-omega-invariant} then imply
        \begin{align}
                         & \ert{\WHILEDO{\kGuard}{C}}{0} (\sigma) \notag \\
                &{}={}~ \lim_{n\to\infty} ~ \left( 1 + \underbrace{\kGuardB (\sigma)}_{{}=1} \cdot \left( \ert{C}{0} (\sigma) \cdot
                             \sum\limits_{i=0}^{n} \underbrace{\wp{C}{\kGuardB} (\sigma)^i}_{{}={}1} ~+~ 
                             \sum\limits_{i=0}^{n-1} \underbrace{\wp{C}{\kGuardB} (\sigma)^i}_{{}={}1} \right) \right) 
                             \tag{by Theorem~\ref{thm:omega-invariants} and  Lemma~\ref{lem:newrule-omega-invariant}} \\
                &{}={}~ \lim_{n\to\infty} ~ 1 + \ert{C}{0} (\sigma) \cdot \sum\limits_{i=0}^{n} 1 ~+~\sum\limits_{i=0}^{n-1} 1
                             \notag \\
                &{}={}~ \lim_{n\to\infty} ~ 1 + \ert{C}{0} (\sigma) \cdot (n+1) +n 
                             \notag \\
                &{}={}~ \infty~. \label{eqn:newrule-proof-casetwo-two-appendix}  
        \end{align}
       Using Theorem~\ref{thm:ert-wp} and Equation~\ref{eqn:newrule-proof-casetwo-two-appendix}, we obtain
       \begin{align*}
                        & \ert{\WHILEDO{\kGuard}{C}}{f} (\sigma) \\
               &{}={}~ \ert{\WHILEDO{\kGuard}{C}}{0} (\sigma) + \wp{\WHILEDO{\kGuard}{C}}{f} (\sigma)     
                            \tag{by Theorem~\ref{thm:ert-wp}} \\
               &{}={}~ \infty + \nkGuardB (\sigma) \cdot f (\sigma)
                            \tag{by Equation~\ref{eqn:newrule-proof-casetwo-two-appendix} and Theorem~\ref{thm:newrule-wpsemantics}(\ref{thm:newrule-wpsemantics-two})} \\
               &{}={}~ \infty \\
               &{}={}~ 1 + \underbrace{\frac{\kGuardB (\sigma) \cdot \left( 1+ \ert{C}{\nkGuardB \cdot f}(\sigma) \right)}{1- \wp{C}{\kGuardB} (\sigma)}}_{{}={}\frac{1}{0} {}\coloneq{}~ \infty} 
 + \nkGuardB (\sigma) \cdot f (\sigma)~.
       \end{align*}
\qed
\end{proof}
\subsection{Proof of Lemma~\ref{lem:apply-rule-relation}}
\label{app:apply-rule-relation}
\subsubsection{Proof of Lemma~\ref{lem:apply-rule-relation}.1}
%\begin{proof}
%      By induction on the structure of $\lBody$.\\ \\
%      \emph{Base case $\lBody = \PASSIGN{\varXI}{\sum\limits_{j=0}^{n} p_j \cdot \langle a_j \rangle}$.} We have
%       $\wp{\lBody}{g} = \RelNewRule{\sum\limits_{j=0}^{n} p_j \cdot g[\varXI / a_j]}{\lBody}$.
%      \\ \\
       %
       %
       %
%       \emph{Induction hypothesis.} Assume that $\RelNewRule{\wp{\lBody}{g}}{\lBody}$ holds for some arbitrary but fixed loop body $\lBody \in \bnl$. \\ \\
       %
       %
       %
%       \emph{Induction step $~\lBody ~\longrightarrow ~ \ITE{\kGuard}{\PASSIGN{\varXI}{\sum\limits_{j=0}^{n} p_j \cdot \langle a_j \rangle}}{\lBody}$.} We have
       %
       %
       %
%       \begin{align*}
%                     &\wp{\ITE{\kGuard}{\PASSIGN{\varXI}{\sum\limits_{j=0}^{n} p_j \cdot \langle a_j \rangle}}{\lBody}}{g} \\
%              &{}={}~ \kGuardB \cdot \wp{\PASSIGN{\varXI}{\sum\limits_{j=0}^{n} p_j \cdot \langle a_j \rangle}}{g} + \nkGuardB \cdot \wp{\lBody}{g} \\
%             &{}={}~ \underbracket{\kGuardB \cdot \sum\limits_{j=0}^{n} p_j \cdot g[\varXI / a_j]}_{\RelNewRule{}{\lBody} ~\text{($\varXI$ does not occur in $\kGuard$)}} 
%                      \qquad +  \underbracket{\nkGuardB \cdot \wp{\lBody}{g} \vphantom{\sum\limits_{j=0}^{n} p_j \cdot g[\varXI / a_j]}}_{\RelNewRule{}{\lBody} ~\text{(by I.H. and $\varXI$ does not occur in $\kGuard$)}}
%       \end{align*}
       %
       %
       %
%       and hence $\RelNewRule{\wp{\ITE{\kGuard}{\PASSIGN{\varXI}{\sum\limits_{j=0}^{n} p_j \cdot \langle a_j \rangle}}{\lBody}}{g}}
%                 {\ITE{\kGuard}{\PASSIGN{\varXI}{\sum\limits_{j=0}^{n} p_j \cdot \langle a_j \rangle}}{\lBody}}$.
%\end{proof}
\begin{proof}
\newcommand{\bxi}[1]{{B_{x_i}}^{#1}}
       We prove a stronger statement: For all sequences $\Blk \in \bnl$ and all $g \in \E$ it holds that 
       \begin{equation}
       \label{eqn:in-proof-lemma-apply-rule-one-to-show}
              \VarsInExp{\wp{\Blk}{g}} ~{}={}~ \VarsInExp{g} \setminus \VarsAssign{\Blk}~.
       \end{equation}       
       It then follows that $\VarsInExp{\wp{\Blk}{g}} \cap \VarsAssign{\Blk} = \emptyset$ and hence $\RelNewRule{\wp{\Blk}{g}}{\Blk}$ by definition.
       Note that every sequence $\Blk \in \bnl$ is of the form $\COMPOSE{\bxi{1}}{\ldots\COMPOSE{}{\bxi{n}}}$  for some $n \geq 1$, where each $\bxi{j}$ is a block.
       Given a program $C \in \pgcl$, let $\VarsGuard{C}$ denote the the set of variables occurring in a guard in $C$. A straightforward induction on the structure of a block
       $B_{x_i} \in \bnl$ yields
       \begin{equation}
              \label{eqn:in-proof-property-block}
              \VarsInExp{\wp{B_{x_i}}{g}} ~{}={}~ \left( \VarsGuard{B_{x_i}} \cup \VarsInExp{g} \right) \setminus \VarsAssign{B_{x_i}}~.
       \end{equation}
       \noindent
       We now proceed by induction on the length of a sequence $n$. \\ \\
       \emph{Induction base}. $\Blk$ consists of a single block $\bxi{1}$. Moreover no guard in $\bxi{1}$ contains a variable since 
       no variable is initialized, i.e.\ $\VarsGuard{C} = \emptyset$. We thus have
       \begin{align*}
              \VarsInExp{\wp{\Blk}{g}} &~{}={}~ \VarsInExp{\wp{{{B_{x_i}}_1}}{g}} \\
              &~{}={}~ \left( \underbracket{\VarsGuard{B_{x_i}}}_{=\emptyset} {}\cup{} \VarsInExp{g} \right) \setminus \VarsAssign{B_{x_i}} 
               \tag{by Equation~\ref{eqn:in-proof-property-block}}\\
              &~{}={}~  \VarsInExp{g} \setminus \VarsAssign{B_{x_i}}~.
       \end{align*} \\
       \emph{Induction hypothesis.} Suppose Equation~\ref{eqn:in-proof-lemma-apply-rule-one-to-show} holds for some arbitrary but fixed sequence $\Blk$ of length $n$ and all $g \in \E$. \\ \\
       \noindent
       \emph{Induction step.} We have 
       \begin{align*}
              &\VarsInExp{\wp{\COMPOSE{\bxi{1}}{\ldots\COMPOSE{\bxi{n}}{\bxi{n+1}}}}{g}} \\
              &{}={}~\VarsInExp{\wp{\COMPOSE{\bxi{1}}{\ldots\COMPOSE{}{\bxi{n}}}}{\wp{\bxi{n+1}}{g}}}
              \tag{by Table~\ref{table:wp}} \\
              &{}={}~ \VarsInExp{\wp{\bxi{n+1}}{g}} \setminus \VarsAssign{\COMPOSE{\bxi{1}}{\ldots\COMPOSE{}{\bxi{n}}}} ~.
              \tag{by I.H.} 
       \end{align*}
       Further, Equation~\ref{eqn:in-proof-property-block} yields 
       \begin{align*}
       \VarsInExp{\wp{\bxi{n+1}}{g}} ~{}={}~ \left( \VarsGuard{\bxi{n+1}} \cup \VarsInExp{g} \right) \setminus \VarsAssign{\bxi{n+1}}~.
       \end{align*}
       Recall that every variable occurring in a guard in $\bxi{n+1}$ must be initialized, that is
       \begin{equation*}
             \VarsGuard{\bxi{n+1}} \subseteq \VarsAssign{\COMPOSE{\bxi{1}}{\ldots\COMPOSE{}{\bxi{n}}}}~.
       \end{equation*}
       Overall, the aforementioned facts and some simple set algebra yields
       \begin{align*}
              &\VarsInExp{\wp{\COMPOSE{\bxi{1}}{\ldots\COMPOSE{\bxi{n}}{\bxi{n+1}}}}{g}} \\
              &{}={}~ \VarsInExp{g} \setminus \VarsAssign{\COMPOSE{\bxi{1}}{\ldots\COMPOSE{\bxi{n}}{\bxi{n+1}}}}~.
       \end{align*}
\end{proof}
\subsubsection{Proof of Lemma~\ref{lem:apply-rule-relation}.2}
\begin{proof}
       %By induction on the structure of $\lBody$. \\ \\
       %
       %
       %
       %\emph{Base case $~\lBody = \PASSIGN{\varXI}{\sum\limits_{j=0}^{n} p_j \cdot \langle a_j \rangle}$.} 
       %We have $\ert{\lBody}{0} = 1 + \sum\limits_{j=0}^{n} p_j \cdot 0[\varXI / a_j] = \RelNewRule{1}{\lBody}$. \\ \\
       %
       %
       %
       %\emph{Induction hypothesis.} Assume that $\RelNewRule{\ert{\lBody}{0}}{\lBody}$ holds for some arbitrary but fixed loop body $\lBody \in \bnl$. \\ \\
       %
       %
       %
       %\emph{Induction step $~\lBody ~\longrightarrow ~ \ITE{\kGuard}{\PASSIGN{\varXI}{\sum\limits_{j=0}^{n} p_j \cdot \langle a_j \rangle}}{\lBody}$.} We have
       %
       %
       %
       %\begin{align*}
       %              &\ert{\ITE{\kGuard}{\PASSIGN{\varXI}{\sum\limits_{j=0}^{n} p_j \cdot \langle a_j \rangle}}{\lBody}}{0} \\
       %       &{}={}~ 1 + \kGuardB \cdot \ert{\PASSIGN{\varXI}{\sum\limits_{j=0}^{n} p_j \cdot \langle a_j \rangle}}{0} + \nkGuardB \cdot \wp{\lBody}{0} \\
       %       &{}={}~ 1 + \underbracket{\kGuardB \cdot \sum\limits_{j=0}^{n} p_j \cdot 0[\varXI / a_j]}_{\RelNewRule{}{\lBody} ~\text{($\varXI$ does not occur in $\kGuard$)}} 
       %               \qquad +   \underbracket{\nkGuardB \cdot \ert{\lBody}{0} \vphantom{\sum\limits_{j=0}^{n} p_j \cdot g[\varXI / a_j]}}_{\RelNewRule{}{\lBody} ~\text{(by I.H. and $\varXI$ does not occur in $\kGuard$)}}
       %\end{align*}
       %
       %
       %
       %and hence $\RelNewRule{\ert{\ITE{\kGuard}{\PASSIGN{\varXI}{\sum\limits_{j=0}^{n} p_j \cdot \langle a_j \rangle}}{\lBody}}{0}}
       %           {\ITE{\kGuard}{\PASSIGN{\varXI}{\sum\limits_{j=0}^{n} p_j \cdot \langle a_j \rangle}}{\lBody}}$.
       We show that $\VarsInExp{\ert{\Blk}{0}} = \emptyset$ holds for every sequence $\Blk \in \bnl$. This implies $\RelNewRule{\ert{\Blk}{0}}{\Blk}$.
       First observe that since every $\Blk \in \bnl$ is loop--free, we have
       \begin{equation}       
              \label{in-proof-lemma-apply-rule-two-wp-ert}
              \VarsInExp{\wp{\Blk}{g}} = \VarsInExp{\ert{\Blk}{g}}~.
       \end{equation}
       Thus Equation~\ref{eqn:in-proof-lemma-apply-rule-one-to-show} verified in the previous proof yields
       \begin{align*}
              \VarsInExp{\ert{\Blk}{0}} &~{}={}~ \VarsInExp{\wp{\Blk}{0}} 
              \tag{by Equation~\ref{in-proof-lemma-apply-rule-two-wp-ert}}\\
              &~{}={}~ \underbracket{\VarsInExp{0}}_{=\emptyset} \setminus \VarsAssign{\Blk} \\
              \tag{by Equation~\ref{eqn:in-proof-lemma-apply-rule-one-to-show}}
              &~{}={}~ \emptyset~.
       \end{align*}
\end{proof}
\input{bn-soundness-proof}
\subsection{Proof of Theorem~\ref{thm:parametrized-loop-runtime}}
\label{proof-thm:parametrized-loop-runtime}
\begin{proof}
Since the expected runtime $\ert{\innerProg}{0}$ of program
$\innerProg$ is a function parameterized by $k$ and $i$, we denote this runtime by $\runC{k}{i} \in \E$. We now propose the following as both a lower and upper $\omega$--invariant of loop
$\outerProg$ w.r.t.\ postruntime $0$ to obtain the program's expected runtime.
\begin{align}
       I_n ~{}={}~ 1 + \sum\limits_{l = 0}^{n} \iverson{x > l} \cdot \left(3 + \iverson{l \neq n} 
                                 + \iverson{l = 0} \cdot \runC{k}{i}
                                 + \iverson{l \neq 0} \cdot \runC{k+l}{1} \right)
                                 \label{eqn:extension-omega-invariant}
\end{align}
In order to verify this, observe the characteristic functional $F_0$ of loop $\outerProg$ w.r.t.\ postruntime $0$, where 
$\outerBody$ denotes the body of loop $\outerProg$:
\begin{align}
                      F_0 (X) &~{}={}~ 1 + \iverson{x > 0} \cdot \ert{\outerBody}{X}
                      \notag \\
       &~{}={}~ 1 + \iverson{x > 0} \cdot \ert{\innerProg}{3 + X[i/1, x/x-1, k/k+1]}
                      \tag{by Table~\ref{table:ert}} \\
       &~{}={}~ 1 + \iverson{x > 0} \cdot \ert{\innerProg}{(3 + X)[i/1, x/x-1, k/k+1]}
                      \notag \\
       &~{}={}~ 1 + \iverson{x > 0} \cdot \left( \runC{k}{i} + (3 + X)[i/1, x/x-1, k/k+1] \right)        
                      \tag{by Equation~\ref{eqn:parametrized-loop-assumption}}    \\
       &~{}={}~ 1 + \iverson{x > 0} \cdot \left(3+ \runC{k}{i} + X[i/1, x/x-1, k/k+1] \right)        
                      \label{eqn:extension-charFunc}                   
\end{align}
We first show $F_0(0) = I_0$. We have
\begin{align*}
                      F_0(0) &~{}={}~ 1 + \iverson{x > 0} \cdot \left(3+ \runC{k}{i} + 0[i/1, x/x-1, k/k+1] \right)  
                      \tag{by Equation~\ref{eqn:extension-charFunc}} \\
       &~{}={}~ 1 + \iverson{x > 0} \cdot \left(3 + \runC{k}{i} \right) \\
       &~{}={}~ 1 + \sum\limits_{l = 0}^{0} \iverson{x > l} \cdot \left(3 + \iverson{0 \neq 0} 
                                 + \iverson{l = 0} \cdot \runC{k}{i}
                                 + \iverson{l \neq 0} \cdot \runC{k+l}{1} \right) \\
       &~{}={}~ I_0~.                          
\end{align*}
Next, we show that $F_0(I_n) = I_{n+1}$ holds:
\begin{align*}
                      F_0(I_n) &~{}={}~ 1 + \iverson{x > 0} \cdot \left(3 + \runC{k}{i} + I_n[i/1, x/x-1, k/k+1] \right)
                      \tag{by Equation~\ref{eqn:extension-charFunc}} \\
       &~{}={}~ 1 + \iverson{x > 0} \cdot \left(3 + \runC{k}{i} + 1 \right. \\
       &\qquad + \sum\limits_{l = 0}^{n} \iverson{x-1 > l} \cdot \left(3 + \iverson{l \neq n} 
                                 + \iverson{l = 0} \cdot \runC{k+1}{1}
                                 + \iverson{l \neq 0} \cdot \runC{k+l+1}{1} \right) \\
       &\phantom{~{}={}~} ) \\
       &~{}={}~ 1 + \iverson{x > 0} \cdot \left(3 + \runC{k}{i} + 1 \right) \\
       &\qquad + \sum\limits_{l = 0}^{n} \iverson{x > l+1} \cdot \left( 3 + \iverson{l \neq n} 
                                 + \iverson{l = 0} \cdot \runC{k+1}{1}
                                 + \iverson{l \neq 0} \cdot \runC{k+l+1}{1} \right) \\
       &~{}={}~ 1 + \iverson{x > 0} \cdot \left(3 + \runC{k}{i} + 1 \right) \\
       &\qquad + \sum\limits_{l = 1}^{n+1} \iverson{x > l} \cdot \left( 3 + \iverson{l \neq n+1} 
                                 + \iverson{l = 0} \cdot \runC{k+1}{1}
                                 + \iverson{l \neq 0} \cdot \runC{k+l}{1} \right) \\     
       &~{}={}~ 1 + \iverson{x > 0} \cdot \left(3 + \runC{k}{i} + 1 \right) 
                         + \sum\limits_{l = 1}^{n+1} \iverson{x > l} \cdot \left( 3 + \iverson{l \neq n+1} 
                                 + \runC{k+l}{1} \right) \\
       &~{}={}~ 1 + \iverson{x > 0} \cdot \left(3 + \runC{k}{i} + \iverson{0 \neq n+1} \right) 
                         + \sum\limits_{l = 1}^{n+1} \iverson{x > l} \cdot \left( 3 + \iverson{l \neq n+1} 
                         + \runC{k+l}{1} \right) 
         \tag{$n \geq 0$}     \\
       &~{}={}~ 1 + \sum\limits_{l = 0}^{n+1} \iverson{x > l} \cdot \left(3 + \iverson{l \neq n+1} 
                                 + \iverson{l = 0} \cdot \runC{k}{i}
                                 + \iverson{l \neq 0} \cdot \runC{k+l}{1} \right)  \\      
       &~{}={}~ I_{n+1}    
\end{align*}
Hence $I_n$ is indeed a lower and upper $\omega$-invariant of loop $\outerProg$ w.r.t.\ postruntime $0$.
Let $I$ denote the same invariant as $I_n$ with n replaced by $\infty$, i.e.
\begin{align*}
        I &~{}={}~ 1 + \sum\limits_{l = 0}^{\infty} \iverson{x > l} \cdot \left(3 + \iverson{l \neq \infty} 
                                 + \iverson{l = 0} \cdot \runC{k}{i}
                                 + \iverson{l \neq 0} \cdot \runC{k+l}{1} \right) \\
          &~{}={}~ 1 + \sum\limits_{l = 0}^{\infty} \iverson{x > l} \cdot \left(4
                                 + \iverson{l = 0} \cdot \runC{k}{i}
                                 + \iverson{l \neq 0} \cdot \runC{k+l}{1} \right) \\
          &~{}={}~ 1 + 4x + \sum\limits_{l=0}^{x-1}  \iverson{l = 0} \cdot \runC{k}{i}
                                 + \iverson{l \neq 0} \cdot \runC{k+l}{1}~.             
\end{align*}
Now, by Theorem~\ref{thm:omega-invariants}, we obtain
\begin{equation*}\label{eqn:extension-runtime-of-Cp}
        \ert{\outerProg}{0} ~{}={}~ I ~{}={}~  1 + 4x + \sum\limits_{l=0}^{x-1}  \iverson{l = 0} \cdot \runC{k}{i}
                                 + \iverson{l \neq 0} \cdot \runC{k+l}{1}~.
\end{equation*}

\end{proof}
\subsection{Complete Calculation of Equation~\ref{eqn:coupoun-harmonic-calculation}}
\label{appendix:coupoun-harmonic-calculation}
We have
\begin{align*}
                 \ert{\couponProg}{0} 
        ~{}={}~& \ert{\couponOuter}{0}[k/0,i/1,x/N] \\
        ~{}={}~& 1 + 5N + \sum\limits_{l=0}^{N-1}  \iverson{l = 0} \cdot  \left(\frac{2 \cdot \iverson{1 \leq 0}}{1 - \frac{1}{N} \cdot  \sum_{j=1}^{N} \iverson{j \leq 0}} \right)          
                                   + \iverson{l \neq 0} \cdot   \left(\frac{2 \cdot \iverson{1 \leq l}}{1 - \frac{1}{N} \cdot  \sum_{j=1}^{N} \iverson{j \leq l}} \right)
                                   \tag{by Theorem~\ref{thm:parametrized-loop-runtime}}  \\
        ~{}={}~& 1 + 5N + \sum\limits_{l=0}^{N-1}  \iverson{l \neq 0} \cdot   \left(\frac{2 \cdot \iverson{1 \leq l}}{1 - \frac{1}{N} \cdot  \sum_{j=1}^{N} \iverson{j \leq l}} \right) \\  
        ~{}={}~& 1 + 5N + \sum\limits_{l=1}^{N-1} \frac{2 \cdot \iverson{1 \leq l}}{1 - \frac{1}{N} \cdot  \sum_{j=1}^{N} \iverson{j \leq l}} \\
        ~{}={}~& 1 + 5N + 2 \cdot \sum\limits_{l=1}^{N-1} \frac{1}{1 - \frac{l}{N}}
                       \tag{$\sum_{j=1}^{N} \iverson{j \leq l} = l$} \\ 
        ~{}={}~& 1 + 5N + 2 \cdot \sum\limits_{l=1}^{N-1} \frac{N}{N-l} \\     
        ~{}={}~& 1 + 5N + 2N \cdot \sum\limits_{l=1}^{N-1} \frac{1}{N-l} \\      
        ~{}={}~& 1 + 5N + 2N \cdot \sum\limits_{l=1}^{N-1} \frac{1}{l}
                       \tag{sum reordering} \\   
        ~{}={}~& 1 + N \cdot \left(5 + 2 \cdot \mathcal{H}_{N-1} \right)~.         
\end{align*}
